# Supplementary material for: On CDCL-based proof systems with the ordered decision strategy
Source: arXiv:1909.04135 source file (2019-09-09)
Supplement: Supplementary file 1 [file appendix.tex]

We  provide comparisons between $\pi$-$P_0$ with ordered resolution and regular resolution, respectively in this Appendix. As is mentioned in Section \ref{sec:main}, they are easy corollaries of Theorem \ref{thm:final} but are much more explicit, so can serve as a warm-up for Theorem \ref{thm:final}.

All restrictions on proofs in this Appendix refer to the usual one, Definition \ref{df:restriction}.
\subsection{v.s. Ordered Resolution: $\oplus$Induction Principle}\label{sec:ind}

\begin{definition}\label{df:ind}
The {\it induction principle} on $n$ variables is the CNF formula $$
Ind(n):=x_1\wedge\bigwedge\limits_{i=1}^{n-1}(x_{i-1}\to x_i)\wedge(\overline{x_n}),\ \ \text{where $x\to y$ means $\overline{x}\lor y$.}$$
$Ind_{\oplus[m]}(n)$ is defined as (the CNF of) the result of substituting each $x_i$ in $Ind(n)$ by $\bigoplus\limits_{u=1}^m y_i^u$, the$\mod 2$ sum of $y_i^1$ to $y_i^m$, where variables $y_i^u$ are new and distinct. 

So $Ind_{\oplus[m]}(n)$ has $mn$ variables, $2^{2(m-1)}(n-1)+2^m$ clauses. We will treat $m$ as a large constant.
\end{definition}

\begin{definition}\label{df:useful orders}
For a $\oplus[m]$-linear variable substitution by $x_i=\oplus_{u=1}^my_i^u$, an order on variables $y_i^u$'s is
\begin{itemize}
\item {\it row-parallel} if $\forall i,j\in[n],u,v\in[m](\ u<v\Leftrightarrow \pi(y_{i}^u)<\pi(y_{j}^v)\ )$;
\item {\it column-parallel} if $\forall i,j\in[n],u,v\in[m](\ \pi(y_{i}^u)<\pi(y_{j}^u)\Leftrightarrow \pi(y_{i}^v)<\pi(y_{j}^v)\ )$.
\end{itemize}
\end{definition}

$Ind(n)$ has an obvious $\pi$-ordered resolution proof of width $4$ and linear size, for {\it any} $\pi$. For $Ind_{\oplus[m]}(n)$ with $m\geqslant 2$, the straightforward refutation is still of linear-size, constant width ($O(m)$), but is only {\it regular} (see \ref{sec:stone}). The following is well-known. For completeness, we include a proof for it in $m=2$ case. The argument works for larger $m$ as well.
\begin{theorem}\label{thm:ind-order}
Let $m\geqslant 2$. Under any row-parallel order, $\pi$-ordered resolutions for $Ind_{\oplus[m]}(n)$ require $O(n)$-width and $2^{O(n)}$-size.
\end{theorem} 

\begin{proof}{(\it{for Theorem \ref{thm:ind-order}, $m=2$})}
Call clauses whose variables belong to $\{y_1^1,...,y_n^1\}$ {\it 1-clauses}. In a $\pi$-ordered refutation $\Pi$, we claim:
$$\text{for any $a=(a_1,...,a_n)\in\{0,1\}^n$, $\exists C$ in $\Pi$ that contains $\bigvee_{i=1}^n(y_1^i)^{1-a_i}$.}$$
To see this, take a restriction $\rho=a$. $\Pi|_\rho$ is a proof of $0$-clause, where the set of non-1 axioms after this restriction form a copy of $Ind(n)$ on variables $y_1^2,...,y_n^2$ (with proper signs), which is a {\it minimal tautology}\footnote{I.e., the absence of any a single axiom results in satisfiability.}. So they must all be used to to derive $0$. Back to $\Pi$, we find a clause $C$ where $y_1^1,...,y_n^1$ (with suitable signs) live from the corresponding axioms to  $C$ as none of them is resolved. The claim follows.  
\end{proof}

On the other hand, there are short $\pi$-$P_0$ refutation for $Ind_{\oplus[2]}(n)$ with parallel orders, as follows.
\begin{theorem}\label{thm:ind}
Under any row- and column-parallel order $\pi$, there is an $O(n^2)$-sized $\pi$-$P_0$ refutation for $Ind_{\oplus[2]}(n)$.
\end{theorem}
\begin{proof}
Denotes by $\oplus(A)$ the group of axioms after $\oplus$-variable substitution of an axiom $A$. We begin with a simple property of $Ind(n)$ for ordered resolution:
\begin{claim}\label{claim:ind}
For any order $\pi'$, there is a $\pi'$-ordered resolution proof of $x_n$ from $Ind_n\backslash\{\neg{x_n}\}$ in size $n$. Symmetrically, there is a $\pi$-ordered resolution proof of $\neg{x_n}$ from $Ind_n\backslash\{x_1\}$ in size $n$.
\end{claim}

Now given a row- and column- parallel order $\pi$, suppose $y_i^2$ is the largest variable under $\pi$. The idea is simple: 
\begin{equation*}
\text{\it Derive $\oplus(x_{i-1}\to x_{i+1})$ so reduce the problem to $Ind_{\oplus[2]}(n-1)$.}
\end{equation*}

{\it Step 1.} By the first part of Claim \ref{claim:ind}, we can make $\pi\text{-ordered}$ resolutions of $O(n)$ steps from $\oplus(x_1),...,\oplus(x_{i-2}\to x_{i-1})$, which resolve only on $y_*^2$ variables (recall $\pi$ is row-parallel) and derive 
\begin{equation}\label{eq:clause}
y_1^1\lor ...\lor y_{i-2}^1\lor (y_{i-1}^1)^a \lor (y_{i-1}^2)^{1-a},\ \ a=0,1.
\end{equation} 
Make the following trails $S^{a,b}$, $a,b\in\{0,1\}$, by consecutive use of Decision rule (note $\pi$ is parallel)
\begin{equation}\label{eq:trail1}
S^{a,b}\text{ as a set is }\{y_j^1\stackrel d =0\mid j\leqslant i-2\}\cup\{y^1_{i-1}\stackrel d =a, y^1_{i+1}\stackrel d=b\}.
\end{equation} 
Use clauses (\ref{eq:clause}) to extend trails (\ref{eq:trail1}) to 
\begin{equation}\label{eq:trail2}
[S^{a,b}, y_{i-1}^2\stackrel u =a],\ \ a,b\in\{0,1\}.
\end{equation}

{\it Step 2.} Apply the second part of Claim \ref{claim:ind} to axioms $\oplus(x_{i+1}\to x_{i+2}),$ ..., $\oplus(\neg{x_n})$, we $\pi$-orderedly derive
\begin{equation}\label{eq:clause2}
(y_{i+1}^1)^a\lor y^1_{i+2}...\lor y^1_n\lor (y^2_{i+1})^a,\ \ a\in\{0,1\}.
\end{equation}
Extend trails (\ref{eq:trail2}) by these clauses to
\begin{equation}\label{eq:trail4}
[S^{a,b}, y^2_{i-1}\stackrel u =a, y^2_{i+1}\stackrel u =1-b],\ \ a,b\in\{0,1\}.
\end{equation}
Finally, extend $(\ref{eq:trail4})$ by Decision rule to
\begin{equation}
T^{a,b,c}:=[S^{a,b},y^2_{i-1}\stackrel u =a, y^2_{i+1}\stackrel u =1-b, y^1_i\stackrel d =c],\ \ a,b,c\in\{0,1\}.
\end{equation}

{\it Step 3.} These $T^{a,b,c}$ can serve as trails (in the Learning rule of $P_0$) for all resolutions between $\oplus(x_{i-1}\to x_i),\ \oplus(x_i\to x_{i+1})$: first $\pi\text{-orderedly}$ resolve on $y^2_i$ and get
\begin{equation}\label{eq:clause3}
(y^1_{i-1})^a\lor (y^2_{i-1})^a \lor (y^1_i)^{c}\lor (y^1_{i+1})^b\lor (y^2_{i+1})^{1-b},\ \ a,b,c\in\{0,1\}.
\end{equation}
Then use state $T^{1-a,1-b,c}$ to resolve on $y^1_i$, between pairs in (\ref{eq:clause3}) of indices $(a,b,0)$, $(a,b,1)$. This produces all clauses in $\oplus(x_{i-1}\to x_{i+1})$. As the result, we get an $Ind_{\oplus[2]}(n-1)$ instance. Recursion on $n$ finishes it. The proof-length is $O(n^2)$.
\end{proof}

\begin{remark}
For $m>2$, the obvious extension of the construction in the proof would fail. So a short and concrete refutation for $Ind_{\oplus[3]}$ requires more careful design (and we better turn to consider Theorem \ref{thm:main}).
\end{remark}

\subsubsection{v.s. Regular Resolution: Stone formulas}\label{sec:stone}
A resolution proof is {\it regular} if it is ``read-once'', i.e., on any path from axioms to root in the refutation, no variable is resolved more than once.
 
Regular resolution is another well-studied subsystem of resolution [{\tt citation needed}]. It is strictly stronger than ordered resolution ( [{\tt citation needed]}; or, $Ind_{\oplus[m]}(n)$ as a quick example).

Our second tautology is the {\it stone formula} (\cite{2007-Alekhnovich-Johannsen-Pitassi-Urquhart} and others). Let $G$ be any directed, acyclic graph with fan-in 2, $n$ vertices, and a single sink vertex; a graph satisfying these conditions is called a {\it pointed graph}. The {stone formula} $Stone(G,S)$\footnote{This is a simplified version, but suffices for our concern.} is a propositional encoding of the following contradictory statement:
\begin{quote} ``All of the source vertices are colored red, the sink is colored blue, and if both the predecessors of a vertex are red, so is the vertex itself.''
\end{quote}

The formal translation is:
\begin{definition}({$Stone(G,S)$})\label{df:stone}
Let $G$ be a pointed graph, where $G = (V,E)$, $|V| = n$, and $S$ is a set of $m\geqslant n$ stones. The variables of the formula $Stone(G,S)$ are $P_{i,u}, i\in V$ and $u\in S$, and $R_v, v\in S$. The variable $P_{i,u}$ says ``Stone $u$ is placed on vertex $i$,'' while $R_v$ says ``Stone $v$ is colored red,'' and $\neg{R_v}$ says
``Stone $v$ is colored blue.''
For a vertex $i\in V$, and a stone $t\in S$, let $D_{i,t}$ be the formula $(P_{i,t}\wedge R_t)$. $Stone(G,S)$ have the following 4 types of clauses:
\begin{enumerate}
\item $\mathop{\bigvee}\limits_{u}P_{i,u},\ \forall i\in V$ (``Every vertex contains some stone'');
\item $P_{k,u}\to R_u,\ \forall u,k\text{ where $k$ is a source of $G$}$;
\item $P_{s,u}\to \overline{R_u},\ \forall j,\text{ and $s$ is the sink of $G$}$;
\item $D_{i,t}\wedge D_{j,u} \wedge P_{k,v} \to R_v,\ \forall i, j, k, t, u, v$ such that $(i,k), (j,k)\in E$. (``If the stones $t,u,v$ are placed on the vertices $i,j,k$, and $t$ and $u$ are both red, then stone $v$ must also be red.')
\end{enumerate}
\end{definition} 

\begin{theorem}[\cite{2007-Alekhnovich-Johannsen-Pitassi-Urquhart}]\label{thm:stone}
For large enough $n$, there exists pointed graph $G$ with $n$ vertices such that, with $|S|=3n$, $Stone(G,S)$ has size lower bound $2^{O(n)}$ for regular resolutions.
\end{theorem}

However, the next theorem says for $\pi$-$P_0$, there is at least {\it some} easy order.
\begin{theorem}\label{thm:stone}
Let $G$ be any a pointed graph on $n$ vertices, and $S$ a set of cardinality $m$. There exists an order $\pi_G$ on variables of $Stone(G,S)$ so that it has $\pi_G$-$P_0$ refutation in size poly$(m,n)$.
\end{theorem}
\begin{proof}
Identify $S$ with $[m]$, and $V(G)$ with $[n]$ so that whenever $(i,j)\in E(G)$, $i$ is smaller than $j$ (which is possible since $G$ is acyclic). So $n$ must be the sink, and $1$ is a source. Let $\pi_G$ be the order under which 
\begin{multline}
P_{n,1}<...<P_{n,m}<P_{n-1,1}<...<P_{n-1,m}<...\\
<P_{1,1}<...<P_{1,m}<R_1<...<R_m.
\end{multline}
The short $\pi_G$-$P_0$ refutation goes by 3 stages. 

1. ({\it Trail preparation}) For any $i<n,l,u\in[m]$, the axiom $P_{n,u} \to \overline{R_ u}$ allows us to build trails where only $({R_u}\stackrel u=0)$ is ``$u$'' , and it is before assignment on $P_{i,l}$.
\\

2. ({\it Induction}) Now use a similar procedure to Lemma 4.1 in \cite{2007-Alekhnovich-Johannsen-Pitassi-Urquhart}, but we stop at vertex $n-1$ rather than $n$. More specifically, we want to inductively derive type 2 clauses, for vertex from sources to $n-1$ (for all stones $u$). We described it here with some emphasis on being $\pi_G$-$P_0$.

For fixed $k<n$, suppose clauses of type 2 have been derived for $i, j(i<j<k)$, where $(i,k),(j,k)\in E(G)$ and for all stones. Derive clauses $(\overline{P_{i,t}}\lor\overline{P_{j,u}} \lor \overline{P_{k,v}}\lor R_v)$ for all $t,u,v\in S$, by resolving axioms of type 2 against appropriate clauses axioms of type 4. These $O(m^3)$ resolutions are simply $\pi_G$-half-ordered. Next we derive clauses $(\overline{P_{j,u}} \lor \overline{P_{k,v}}\lor R_v)$ for all $u,v\in S$, by resolving the previously obtained clauses with type 1-axioms on $i$. To be in $\pi$-$P_0$, we do it in $t$-decreasing order: for all $u,v\in S$, the first resolution
$$\binaryinf{\overline{P_{i,m}}\lor\overline{P_{j,u}}\lor \overline{P_{k,v}}\lor R_v}{\lor_{t\leqslant m}P_{i,t}}{\lor_{t\leqslant m-1}P_{i,t}\lor\overline{P_{j,u}}\lor \overline{P_{k,v}}\lor R_v}
$$
is simply $\pi_G$-half-ordered; while for $t=m,...,1$ in order,
$$\binaryinf{\lor_{l \leqslant t} P_{i,l} \lor \overline{P_{j, u}} \lor \overline{P_{k,v}}\lor R_v}{\overline{P_{i,t}} \lor \overline{P_{j,u}}  \overline{P_{k,v}}\lor R_v}{\lor_{l \leqslant t-1}\lor P_{i,l}\lor \overline{P_{j, u}}  \overline{P_{k,v}}\lor R_v}\ (\text{resolve on $P_{i,t}$})$$ 
uses suitable trails prepared in step 1, which have $(P_{i,t}\stackrel *=0)$ as end (note $i<n$) and proper variable assignments. In the end, we get $(\overline{P_{j,u}}\overline{P_{k,v}}\lor R_v)$ for all $u,v$, in $O(m^3)$ steps. Repeat this on these newly got clauses, we further derive $(\overline{P_{k,v}}\lor R_v), \forall v$.
\\

3. ({\it Clear-up}) {\it All resolutions in this step will be $\pi_G$-half-ordered}. Resolve above $\overline{P_{n-1,t}} \lor R_t$ with axiom $\overline{P_{n-1,t}} \lor \overline{R_t} \lor \overline{P_{n,u}} \lor R_{u}$; and further its result with axiom $P_{n,u} \to \overline{R_ u}$, get 
$$\overline{P_{n-1,t}} \lor \overline{P_{n,u}},\ \forall t,u.$$
Call such a clause $A_{t,u}$. Resolve them with axioms $\lor_{t} P_{n-1,t}$ in decreasing order on $t$:
\begin{equation*}
\begin{aligned} 
Res(\lor_{t\leqslant m} P_{n-1,t},\ A_{m,u})=&\text{ clause we call }C_{m-1,u},\\
Res(C_{m-1,u},\ A_{m-1,u})=&\text{ clause we call }C_{m-2,u},\\
...&\\
Res(C_{1,u},\ A_{1,u})=&\ \overline{P_{n,u}},
\end{aligned}
\end{equation*}
for all $u$. Finally, $\overline{P_{n,u}}$ resolve with axioms $\lor_u P_{n,u}$ in order $u=m,m-1,...,1$, to $0$.
\end{proof}
\begin{remark}\label{rmk:p2}
Another aspect of simplicity of the $P_0$-proof above: all trails used are only generated from axioms. In other words, it falls in the sub-system of $\pi$-$P_0$ which additionally inhibits unit propagation after the first resolution step. Therefore, even such sub-system\footnote{which is complete for refutation, as it contains ordered resolution.} is not outperformed by regular resolution w.r.t. all orders. Although this sub-system can be easily fooled by adversary orders.\footnote{Let $\tau'$ be a hard tautology for ordered resolution. $\tau:=\{A\lor y\lor z\mid A\in\tau'\}\cup\{y\lor \overline{z}, \overline{y}\lor z,\overline{y}\lor\overline{z}\}$ where $y,z$ are new. Let $\pi$ make $y,z$ the largest two. Then $\tau$ is hard for such system with order $\pi$.}
\end{remark}
